# Supplementary material for: The stabilizing effect of volatility in financial markets
Source: arXiv:1708.08695 ancillary file (2017-08-29)
Supplement: Supplementary file 1 [file Supplemental_Material.pdf]

# SUPPLEMENTARY MATERIAL

## for "The stabilizing effect of volatility in financial markets"

Davide Valenti[1], Giorgio Fazio[2,3], Bernardo Spagnolo[1,4]

[1] *Dipartimento di Fisica e Chimica, Group of Interdisciplinary Theoretical Physics and CNISM, Università di Palermo, Viale delle Scienze, edificio 18, I-90128 Palermo, Italy*

[2] *Business School, Newcastle University, 5 Barrack Road, NE1 4SE, Newcastle upon Tyne, UK*

[3] *SEAS, Università di Palermo, Italy*

[4] *Istituto Nazionale di Fisica Nucleare, Sezione di Catania, Italy*

### I. FIRST HITTING TIME

The *first hitting time* (FHT) is defined as the time it takes for a variable to cross for the first time a certain level. In Fig. S1 we show the schematic representation of the FHT calculated starting from the time series of returns.

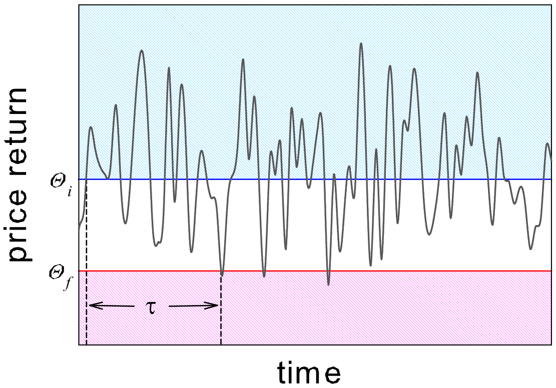


Figure S1. Time series of returns and the corresponding first hitting time, that is the time it takes for a stock price return to cross for the first time a large negative threshold $\Theta_f$ starting from an initial position $\Theta_i$. By ensemble averaging on all the time series of the market we obtain the proposed indicator of price return stability.

The mean first hitting time (MFHT), or mean first passage time (MFPT), was earlier introduced in scientific literature. Indeed, the study of first-passage time and exit problem has a long and standing tradition in physics, mathematics, engineering, and natural sciences. The first pioneering papers in this subject are those by Smoluchowski, who first considered the problem of the random walk with reflecting and absorbing barriers [S1]; Pontryagin *et al.* who first derived the differential equation for the mean first passage time [S2]; Kramers, with his celebrated paper on "Brownian motion in a field of force and the diffusion model of chemical reactions" [S3], who understood well the mechanism of the escape process as a noise-assisted reaction; S. Chandrasekhar, who considered the importance of the occurrence of the escape problem in astronomical phenomena [S4]; W. Feller, who gave his fundamental contribution in mathematical literature, with his proposal of two singular diffusion problems, called Feller processes, and the related boundary problem appearing in these diffusion processes [S5, S6]. Indeed, the fact that the Feller process never attains negative values has made it an ideal candidate for modeling many natural and social science phenomena.

### II. THE HESTON MODEL

The Heston model [S7–S10], which describes the dynamics of stock prices $p(t)$ as a geometric Brownian motion with the volatility given by a mean-reverting process, known as Cox, Ingersoll, and Ross (CIR) process [S10–S13], is defined by the following Itô stochastic differential equations

$$dp(t) = \mu\ p\ dt + \sigma(t)p\ dW_1(t) \tag{S1}$$
$$dv(t) = a(b - v(t))\ dt + c\ \sqrt{v(t)}\ dW_2(t), \tag{S2}$$

where $\sigma(t)$ is the time-dependent volatility, $v(t) = \sigma^2(t)$ and $W_i(t)$ are uncorrelated Wiener processes with the usual statistical properties

$$< dW_i >= 0, \; < dW_i(t) dW_j(t') > = \; dt \; \delta(t - t') \; \delta_{i,j}. \tag{S3}$$

The CIR process, known in mathematical statistics as the Feller process [S5], and later introduced in mathematical finance [S12], represents the term structure of interest rates and it successfully evaluates bond prices [S12, S13]. Moreover, the Feller process also appears to describe the default intensity rate [S14], and the growth stock [S15]. Stochastic volatility obeying the Feller model jointly with a log-Brownian stochastic dynamics for the asset price evolution gives rise to a two-dimensional diffusion market process called the Heston model [S7, S8], which is a useful model for option pricing [S7, S10, S13]. Recently, a study of the mean first passage time (MFPT) (or mean first hitting time (MFHT)) for two well-known mean-reverting processes, that is the square root process of Feller and the GARCH diffusion process, was done in Refs. [S10] and [S16]. Specifically, in [S16], the asymptotic expansions of the MFPT around the starting position and the boundary points of GARCH and Feller processes as well as the sensitivity analysis of MFPT to changes of relevant parameters were investigated. In Ref. [S10], the first-passage and escape problems for the Feller process have been fully addressed. Moreover, we note that the square root process of Feller is connected to the square of a $\delta$-dimensional Bessel process [S17].

In Eq. (S1) $\mu$ represents a drift at macroeconomic scales. In Eq. (S2) the volatility $\sigma(t) = \sqrt{v(t)}$ reverts towards a macroeconomic long time term given by the mean squared value $b$, with a relaxation time $a^{-1}$. Here $c$ is the amplitude of volatility fluctuations often called the *volatility of volatility*.

By introducing log-returns $x(t) = ln(p(t)/p(0))$ in a time window $[0, t]$ and using Itô's formula [S21], we obtain the stochastic differential equation (SDE) for $x(t)$

$$dx(t) = (\mu - v(t)/2) \; dt + \sqrt{v(t)} \; dW_1(t). \tag{S4}$$

We note that the Heston model gives a good reproduction of the price returns probability density function (PDF), but does not reproduce long-range volatility correlation [S18]. On the contrary, the GARCH model provides a basic way to model volatility correlation, modeling the high memory of the volatility [S20], but gives a rather poor fitting of the return PDF (see Refs. [S18–S20]). Moreover, the statistical properties of the returns and FPTs for models with stochastic volatility, such as the Heston and the discrete GARCH (1,1) model, have been investigated in Refs. [S18, S19], finding that the PDF of both stock price returns and FPTs obtained with the Heston model exhibit a better agreement with real market data than those calculated in the GARCH discrete model.

## III. THE NONLINEAR HESTON MODEL

Here we consider a generalization of the Heston model, by replacing the geometric Brownian motion with a random walk in the presence of a cubic nonlinearity [S11]. This generalization represents a fictitious "*Brownian particle*" moving in an *effective* potential with a metastable state given by $U(x) = Ax^3 + Bx^2$. The proposed nonlinear Heston model is defined by the following Itô stochastic differential equations [S21]

$$dx(t) = -\left(\frac{\partial U}{\partial x} + \frac{v(t)}{2}\right) dt + \sqrt{v(t)}\, dW_1(t), \tag{S5}$$

$$dv(t) = a[b - v(t)]\, dt + c\, \sqrt{v(t)}\, dW_2(t), \tag{S6}$$

with the volatility $v(t)$ given by the mean-reverting CIR process [S5, S8, S12, S13]. Here, $x(t) = ln[p(t)/p(0)]$ is the return and $W_i$ are uncorrelated Wiener processes.

Some of the well-established statistical properties of the financial time series are the PDFs of stock price returns and volatility, the return correlation, and the absolute return correlation. In the following Fig. S2 we show the PDF of the stock price returns for real data (blue circles) and model (red triangles). We find that the agreement between theoretical results and real data of the PDFs of returns is quite good, except at high values of the returns. This can be ascribed to the failure of the proposed nonlinear model for returns higher or comparable to the height of the metastable state barrier (see Ref. [63] of the main article). To quantitatively characterize the PDF of returns (Fig. S2) with respect to their average, width, asymmetry, and fatness, we consider the whole set of $N_T$ values of the daily returns and calculate, both for real data and theoretical results, the four moments of the PDF, that is the mean value

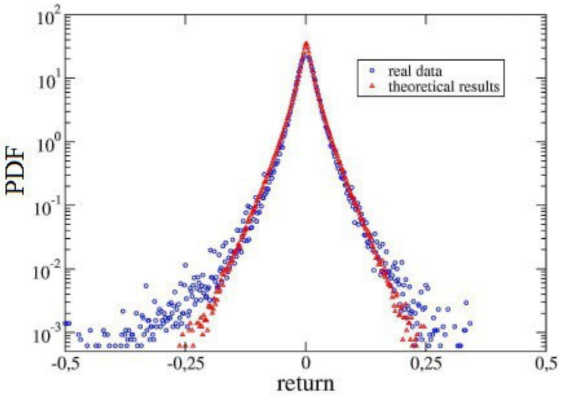


Figure S2. PDF of the stock price returns for real data (blue circles) and model (red triangles).

$< r >$, the variance $\sigma_r$, the skewness $\kappa_3$, and the kurtosis $\kappa_4$, obtaining the following values: $< r >^{exp} = -1.91 \cdot 10^{-5}$, $\sigma_r^{exp} = 0.025$, $\kappa_3^{exp} = -4.30$, and $\kappa_4^{exp} = 442$, and $< r >^{theor} = -4.76 \cdot 10^{-5}$, $\sigma_r^{theor} = 0.024$, $\kappa_3^{theor} = -1.96$, and $\kappa_4^{theor} = 105$. The quantitative statistical characterization of the shape of the PDF of returns shows that the model reproduces the asymmetry and leptokurtic distribution observed for the real market data.

In Fig. S3a we show the PDF of the volatility both for real market data and theoretical results, finding a log-normal behavior in both cases. The agreement is quite good, as confirmed by the Kolmorogov-Smirnov test: $D = 0.2178$ and $P = 0.014$. Here, $D$ and $P$ are respectively the maximum difference between the cumulative distributions and the corresponding probability for the K-S test.

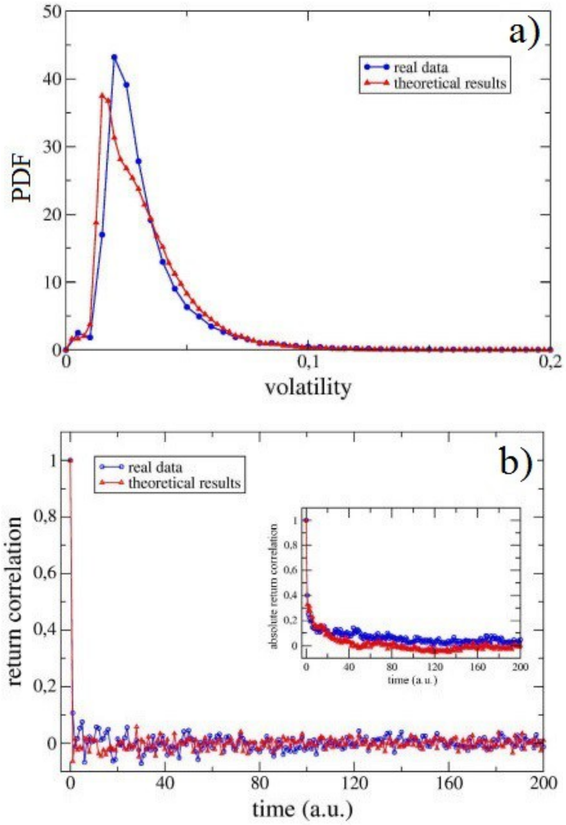


Figure S3. a) Probability distribution of the volatility for real data (blue circles) and model (red triangles). We consider the whole set of price returns consisting of $N_T = 3030 \times 1071 = 3245130$ values and calculate, both for real data and theoretical results, the related PDFs. b) Correlation function of the returns for real data and model. Inset: Correlation function of the absolute returns for real data and model. The values of the parameters are the same as in Fig. 3 of the main article.

The values of the volatility shown in Fig. S3a are those corresponding to the hitting time events observed for $\Theta_i = -0.1\bar{\sigma}^r$ and $\Theta_f = -1.5\bar{\sigma}^r$ (see Fig. 1a of the main article).

In Fig. S3b we show the autocorrelation function of the asset returns, calculated by our nonlinear Heston model (Eqs. S5 and S6) (red triangles), and compared with that obtained from the real data (blue circles). We note absence of return autocorrelation (see Ref. [65] in the main article).

Finally, we note that the "*clustering*" phenomenon of volatility is important for understanding the instabilities in price returns. We had clear evidence of this phenomenon looking at the time series of the returns used in our empirical analysis. Moreover, the contemporaneous presence, in the time series of returns, of "*clustering*" and "*spikes*" of volatility gives rise to the nonmonotonic behavior observed in Figs. 1 and 2 of the main article. Specifically, the simultaneous presence of two neighboring spikes is correlated with the presence of low MFHTs at low volatility, while a spike close to a cluster is related to low MFHTs at high volatility values. Pairs of clusters and/or spikes spaced from a nearly laminar or "tranquil" regime give rise to an increase of the MFHT (intermediate region of volatility values) with the presence of a maximum. This gives rise to the observed nonmonotonic behavior of the MFHT vs volatility.

[S1] M. v. Smoluchowski, Physik. Zeits. **17**, 557 (1916).
[S2] L. S. Pontryagin, A. A. Andronov and A. A.Witt, J. Exsp. Teor. Fiz. **3**, 165 (1933).
[S3] H. A. Kramers, Physica **7**, 284 (1940).
[S4] S. Chandrasekhar, Rev. Mod. Phys. **15**, 1 (1943).
[S5] W. Feller, Ann. Math. **54**, 173 (1951).
[S6] W. Feller, Ann. Math. **55**, 468 (1952).
[S7] S. L. Heston, Rev. Financ. Stud. **6**, 327 (1993).
[S8] A. A. Dragulescu and V. M. Yakovenko, Quant. Fin. **2**, 443 (2002).
[S9] J. Masoliver, J. Perelló, Phys. Rev. E **80** 016108 (2009); Phys. Rev. E **78**, 056104 (2008).
[S10] J. Masoliver, J. Perelló, Phys. Rev. E **86** 041116 (2012).
[S11] G. Bonanno, D. Valenti, B. Spagnolo, Phys. Rev. E **75**, 016106 (2007).
[S12] J. C. Cox, J. E. Ingersoll, and S. A. Ross, Econometrica **53**, 385 (1985).
[S13] J. C. Hull, *Options, Futures, and Other Derivatives* (Prentice Hall, London, 2011).
[S14] D. Duffie, and K. Singleton, Rev. of Financ. Stud. **12**, 687 (1999).
[S15] S. Kou, and S. G. Kou, Math Oper. Res. **29**, 191 (2004).
[S16] Bo. Zhao, *Mean first-passage times of the Feller and the GARCH diffusion processes*, https://urlsand.esvalabs.com/?u=httpCity University London - Sir John Cass Business School. Cass Business School, London (2010).
[S17] J. Pitman and M. Yor, Z. Wahrscheinlichkeit **59**, 425 (1982)
[S18] G. Bonanno and B. Spagnolo, Fluct. Noise Lett. **5** (2), L325 (2005).
[S19] D. Valenti, B. Spagnolo, G. Bonanno, Physica A **382**, 311 (2007).
[S20] J. Gatheral, *Consistent modeling of SPX and VIX options*, Technical report. Merrill Lynch, 2008.
[S21] C. W. Gardiner *Handbook of Stochastic Methods*, (Springer, Berlin, 2004).
